# Supplementary material for: Nernst effect and dimensionality in the quantum limit
Source: arXiv:0909.2137 source file (2009-09-11)
Supplement: Supplementary file 1 [file Supplmentaryinformation.pdf]

# Supplementary information for “Nernst effect and dimensionality in the quantum limit”

Zengwei Zhu[1,2], Huan Yang[1], Benoît Fauqué[1], Yakov Kopelevich[3] and Kamran Behnia[1]

[1] Laboratoire de Photons et matière (CNRS-UPR5), ESPCI, 10, Rue Vauquelin, 75231 Paris, France
[2] Department of Physics, Zhejiang University, Hangzhou 310027, China
[3] Instituto de Fisica ``Gleb Wataghin'', Universidade Estadual de Campinas, UNICAMP, 13083-970 Campinas, São Paulo, Brazil

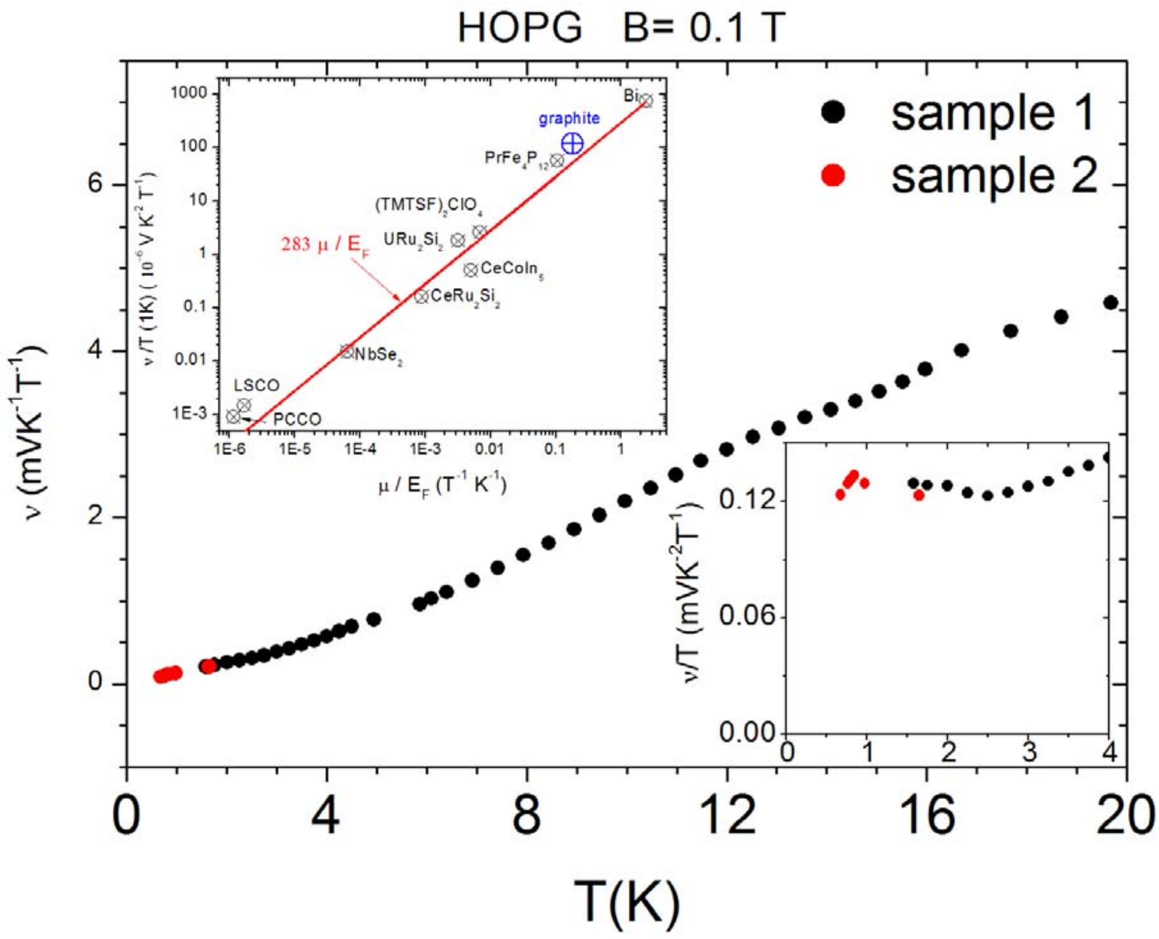


**Fig. S1:** The main panel shows the temperature dependence of the Nernst coefficient of the two HOPG samples. The lower inset presents a zoom on the temperature dependence of ν/T below 4K. In the upper inset, the extracted value for ν/T is compared with other systems using a figure from ref. S1.

## Method of measurement

The Nernst effect was measured with a two-thermometer-one-heater set-up. One end of the sample was anchored to the cold finger and a heat current was applied along

the sample with a heater. Thermal gradient across the sample and the average temperature of the sample in presence of the heat current were measured with two thermometers. The set-up for low temperatures used $RuO_2$ thermometers and cernox thermometers were used in the other set-up designed to work at T>1.2 K. Our set-up allowed us to measure the four transport coefficients, $\rho_{xx}$, $\rho_{xy}$, $S_{xx}$ and $S_{xy}$ with the same contacts and in the same conditions.

## Magnitude of the Nernst coefficient in graphite

Fig. S1 shows our data for the temperature dependence of the Nernst coefficient, $\nu$, in presence of a small field (B=0.1 T) in the two HOPG samples studied in this work. The asymptotic slope of $\nu$ in the zero-temperature limit can be extracted by plotting $\nu/T$ at low temperatures. The only previous report on the Nernst effect in graphite, of which we are aware, is restricted to temperatures above the liquid nitrogen[S1].

As expected for an ambipolar semi-metal [S2, S3], the Nernst effect in graphite is large and as can be seen in the upper inset of the figure, elemental bismuth is the only metal to present a larger $\nu$ [S2]. In order to determine the position of graphite in this panel, the Fermi energy was taken to be 19 meV [S4] and the mobility of the samples (~3 $10^5$ $cm^2V^{-1}s^{-1}$) used in this study was estimated using their resistivity ratio compared to those measured by Soule [S5].

## Quantum oscillations in Nernst and Seebeck responses

Fig. S2 compares the oscillations of the Nernst and Seebeck coefficients at two different temperatures. As seen in the figure, there is a shift between the position of maxima in the two sets of data. Maxima in $S_{xy}$ are concomitant with a sign change in $S_{xx}$. Peaks of the Nernst signal are indexed as detailed below. There is no noticeable difference between the profile of the $S_{xy}$ response of hole-like carriers and electron-like carriers.

In the case of $S_{xx}$, on the other hand, the anomalies for one type of carriers (those indexed L (with a frequency of 6.5 T) are weaker than those indexed S (with a frequency of 4.6 T). This may result from the difference between the energy dispersion in the two cases. However, the profile of $S_{xx}$ anomaly is the same for the two pockets and is not influenced by the hole-like or the electron-like nature of the carriers.

## Indexing Landau levels

Nernst peaks could be easily identified, following a previous study by Woollam [S6] based on the theoretical prediction by Sugihara and Ono [S7]. The latter authors assumed that the carriers of the pocket near the point H are electrons and those associated with the pocket near the point K are holes. On the other hand, the analysis of the magnetoreflection data led Schroeder *et al.* [S8] to revise the original SWM model [S9, S10] and suggest the opposite: electrons were now believed to be at point K and holes at point H. Most authors are currently following this assumption [S11, S12] and consider the carriers of the larger pocket to be electron-like and those on the smaller one to be holes. On the other hand, Luk'yanchuk and Kopelevich,

comparing the phase shift of the dHvA and SdH oscillations concluded that the high-frequency carriers are holes and low-frequency carriers are electrons, [S13, S14].

The Nernst peaks and the indexes of their corresponding Landau levels are presented in Fig S2. We use L and S for Large and Small pockets regardless of the sign of their carriers, since this issue cannot be settled by our thermomagnetic data.

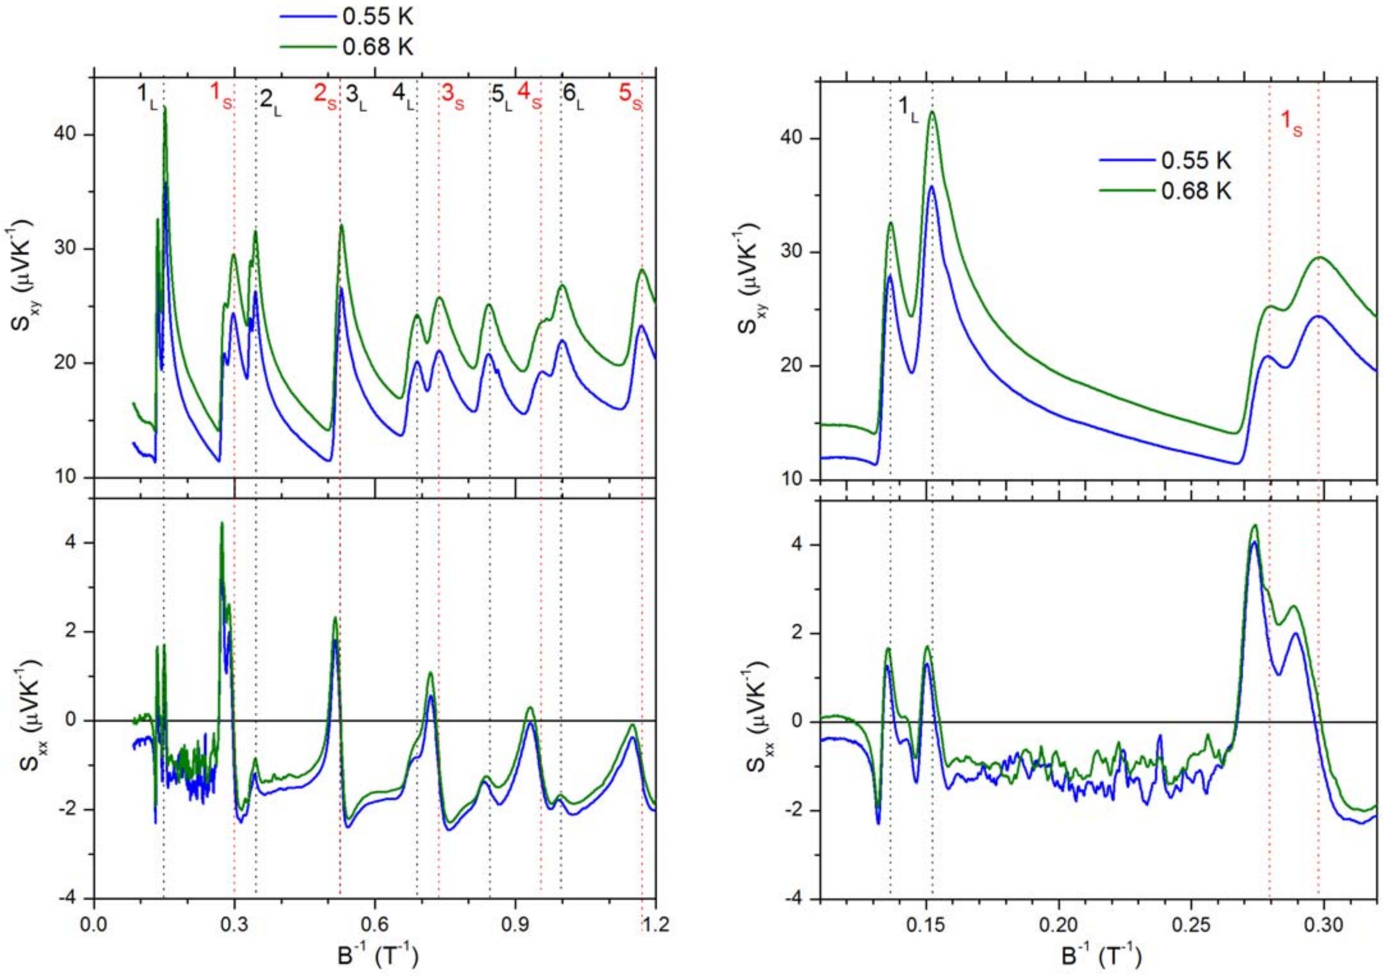


**Fig.S2:** Left panel: Nernst (top) and Seebeck (bottom) effects as a function of inverse of magnetic field for two different temperatures. Dotted verical lines mark the position of peaks in the Nernst response. The Nernst peaks are concomitant with a more complex structure (a minimum adjacent to a maximum) in the Seebeck response. Right Panel is a zoom on the high-field region.

Fig. S3a is a plot of the inverse field position of the Landau levels as a function of their quantum numbers. As seen in the figure, our data points are almost identical to what has been reported very recently by Schneider *et al.* who performed a high-resolution magnetoresistance study [S12].

There is no noticeable experimental discrepancy between these data points and those reported by Luk'yanchuk and Kopelevich [S14,S15] who have recently suggested a non-trivial Berry phase for the carriers of the one of the two Fermi surface pockets [S13-S15]. Indeed, as seen in the figure, a linear extrapolation of the

data points leads to very different intercepts for the two pockets, suggesting a different Berry phase.

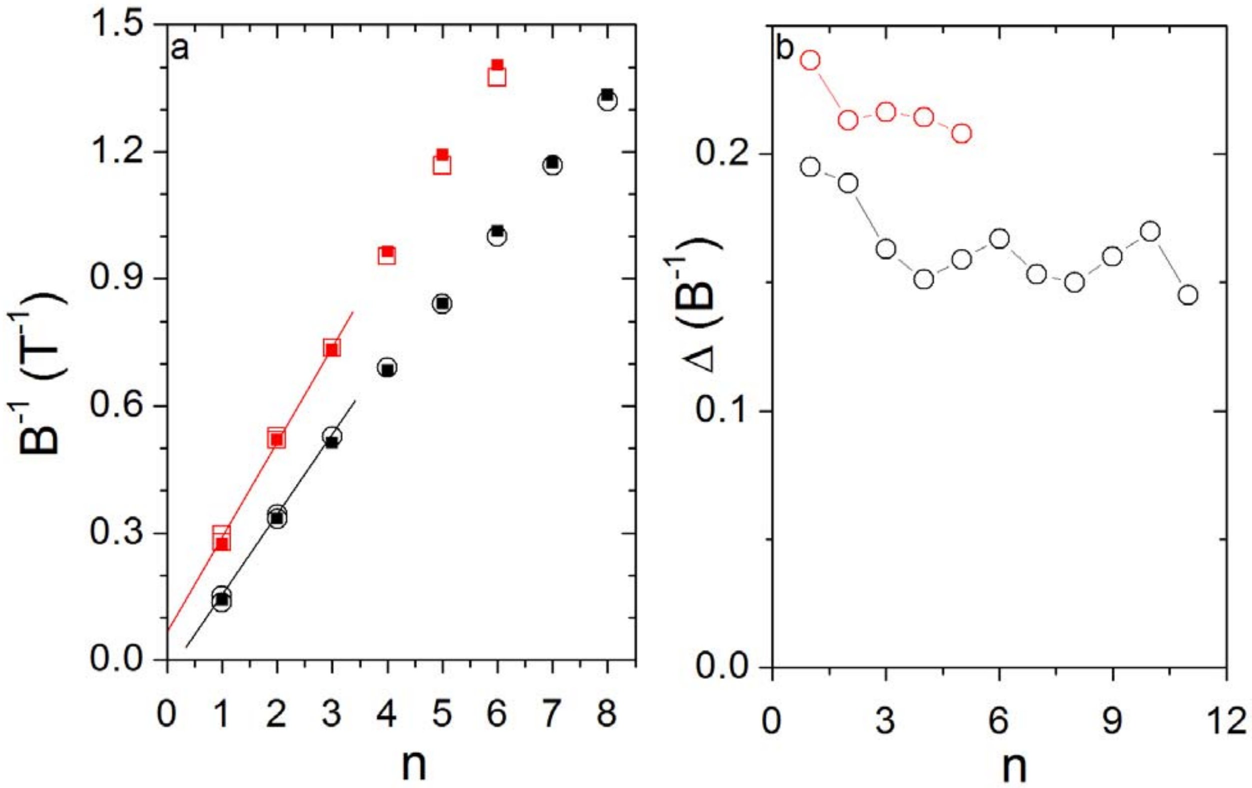


**Fig.S3:** a) The field position of identified Nernst peaks (open symbols) of the two pockets as a function of their quantum numbers. The solid symbols represent the same for the minima in $\rho_{xx}$ according to the data reported by Schneider *et al.* in ref. S11. A linear extrapolation would lead to different intercepts for the two pockets. b) The period, defined as the distance between two successive peaks in $B^{-1}$, as a function of their index numbers. The field-induced modification of the Fermi level gives rise to ripples. Red (black) symbols correspond to quantum oscillations of the smaller (larger) Fermi pocket.

This proposition has provoked an ongoing debate [S11-S15]. In particular, Schneider *et al.* [S12], invoking the field-induced variation of the Fermi energy, conclude that the conventional SWM picture is sufficient to explain the data. Fig. S3b presents the period as a function of the quantum number. If the carrier density were fixed, these values would be constant and the points would fall along a horizontal line. The ripples are a consequence of the continuous adjustment of the Fermi energy with field in order to keep charge neutrality [S7]. It is yet to be demonstrated that this variation suffices to explain the striking phase shift seen in the right panel of Fig. S3.

## HOPG and natural graphite

Graphite natural single crystals are known to be different from HOPG samples in a number of their physical properties. In particular, since the zero-field anisotropy of electric conductivity can be two orders of magnitude larger in HOPG samples than in natural graphite, it has been suggested that the former is more quasi-two-dimensional than the latter [S16].

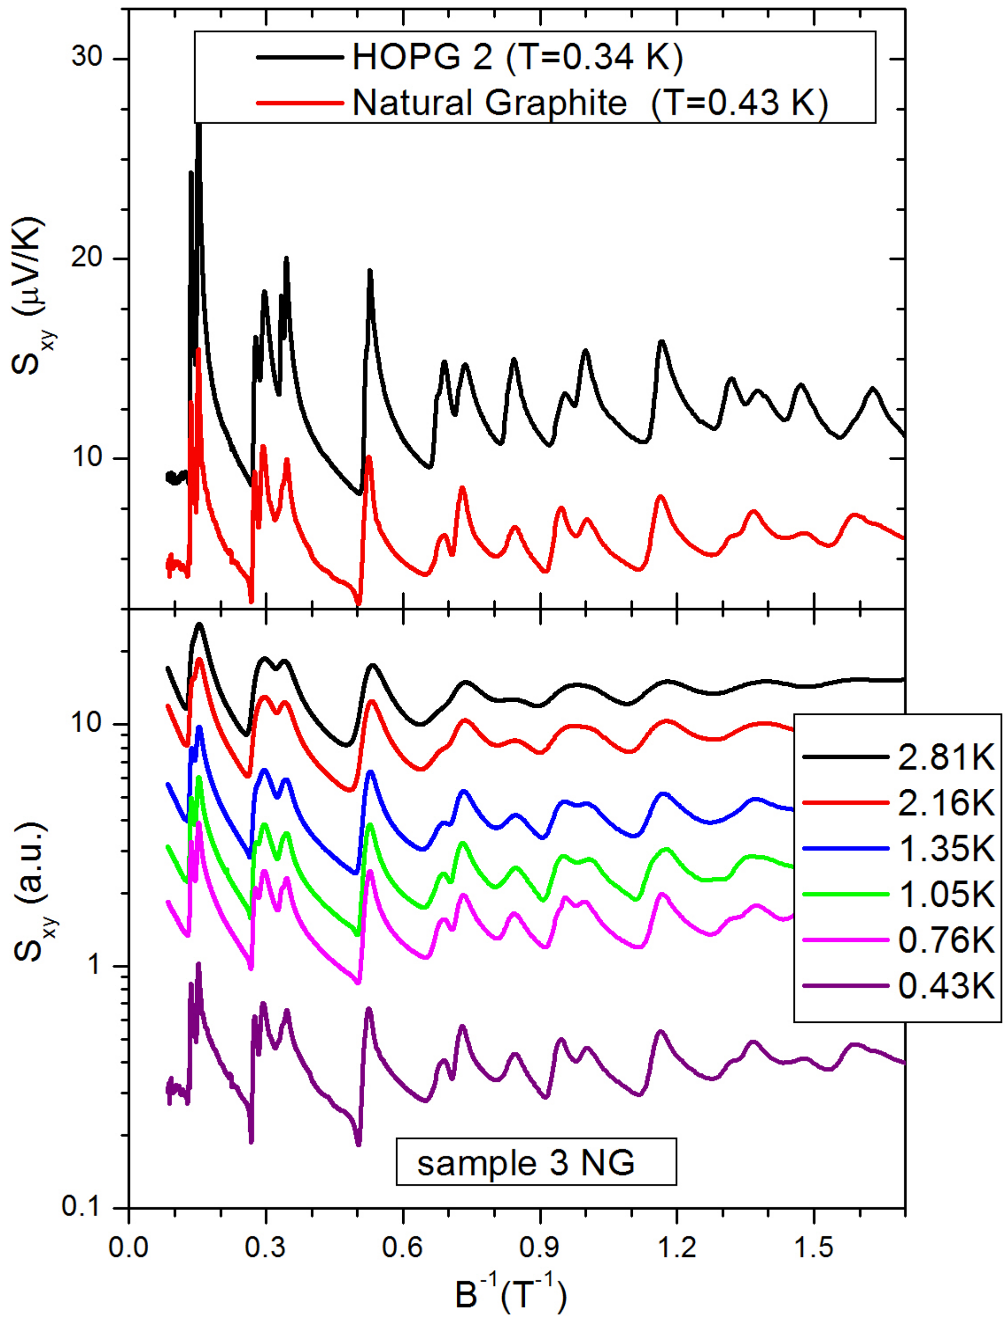


**Fig. S4:** Upper panel: Comparison of the structure and the magnitude of the Nernst signal in a HOPG sample and a natural graphite single crystal. Lower panel: The temperature evolution of the Nernst signal in the natural graphite single crystal.

In order to see if there is a difference in their Nernst response, we measured the Nernst signal of a natural single crystal. The results are presented in Fig. S4. As seen in the figure, the difference between the two sets of data is marginal. The magnitude of the Nernst signal in the HOPG sample is twice higher. Moreover, in the natural crystal, the amplitude of one of the S pocket decays faster with decreasing magnetic

field pointing to a lower mobility of the carriers associated with this pocket. In spite of these minor differences, the field position and the profile of the Nernst peaks are quasi-identical.

## References


**S1.** J. J. Mills, R. A. Morant and D. A. Wright, Brit. J. Appl. Phys. **16**, 479 (1965).
**S2.** K. Behnia, J. Phys.: Condens. Matter, **21**, 113101 (2009).
**S3.** A. A. Varlamov and A. V. Kaovokin, Europhys. Lett., **86** , 47007 (2009).
**S4.** N. B. Brandt, S. M. Chudinov and Ya. G. Ponomarev, Semimetals I. Graphite and its compounds (Elsevier, Amsterdam 1988).
**S5.** D. E. Soule, Phys. Rev. **112**, 698 (1958).
**S6.** J. A. Woollam, Phys. Rev. B **3**, 1148 (1971).
**S7.** K. Sugihara and S. Ono, J. Phys. Soc. Jpn. **21**, 631 (1966).
**S8.** P. R. Schroeder, M. S. Dresselhaus and A. Javan, Phys. Rev. Lett., **20**, 1292 (1968).
**S9.** J. C. Slonzewski and P. R. Weiss, Phys. Rev. **109,** 272 (1958).
**S10.** J. W. McClure, Phys. Rev. **108**, 612 (1957).
**S11.** G. P. Mikitik and Yu. V. Sharlai, Phys. Rev. B **73**, 235112 (2006).
**S12.** J. M. Schneider, M. Orlita, M. Potemski and D. K. Maude, Phys. Rev. Lett. **102**, 166403 (2009).
**S13.** I. A. Luk'yanchuk and Y. Kopelevich, Phys. Rev. Lett. **93**, 166402 (2004).
**S14.** I. A. Luk'yanchuk and Y. Kopelevich, Phys. Rev. Lett. **97**, 256801 (2006).
**S15.** I. A. Luk'yanchuk and Y. Kopelevich, ArXiv:0907.2026
**S16.** Y. Kopelevich and P. Esquinazi, Adv. Mater. **19**, 4559 (2007).
